# Supplementary material for: Phylogenetic signal in phonotactics
Source: arXiv:2002.00527 source file (2020-07-14)
Supplement: Supplementary file 1 [file supplementary_information.pdf]

# Supplementary Information

## Phylogenetic signal in phonotactics

Jayden L. Macklin-Cordes, Claire Bowern, Erich R. Round

## S1. Pama-Nyungan reference phylogeny

Quantifying phylogenetic signal requires an independently-derived reference phylogeny as a yardstick. Our reference phylogeny is a 285-tip Pama-Nyungan phylogeny inferred by the second author. Figure S1 gives a 111-tip subset of this phylogeny, corresponding to the 111 doculects used in this study.

As discussed in the main paper, the reference phylogeny was constructed using Bayesian phylogenetic methods in the software BEAST2 (Bouckaert et al. 2014). Bayesian phylogenetic methods use a Markov Chain Monte Carlo (MCMC) procedure to efficiently search the hypothesis space of possible trees and return a large posterior sample of similarly credible alternatives (capturing phylogenetic uncertainty). The tree in Figure S1 above is a maximum clade credibility tree, which is a summation of the posterior sample where the likelihood of all nodes in the tree (in terms of how frequently a given node reappears across the posterior sample) is maximized.

For further details on the Pama-Nyungan phylogeny used as a reference phylogeny in this study, see Bowern (2015). See also Bowern & Atkinson (2012), which infers a Pama-Nyungan phylogeny in the same way, using exactly the same evolutionary model parameters, but with an earlier iteration of the dataset containing fewer doculects. Additional discussion of the general process of constructing language phylogenies in BEAST2 can be found in Bouckaert, Bowern & Atkinson (2018), although a different evolutionary model is used.

The reference phylogeny was inferred using lexical cognate data, coded according to the principles of the Comparative Method. The cognate data used in the reference phylogeny is publicly available on Zenodo (Bowern 2018) and also as a subset of the 305-language dataset in Bouckaert, Bowern & Atkinson (2018). This latter source also includes a Perl script for converting multistate cognate judgements into a binary matrix for use with BEAST2 phylogenetic software and will include information on underlying sources.

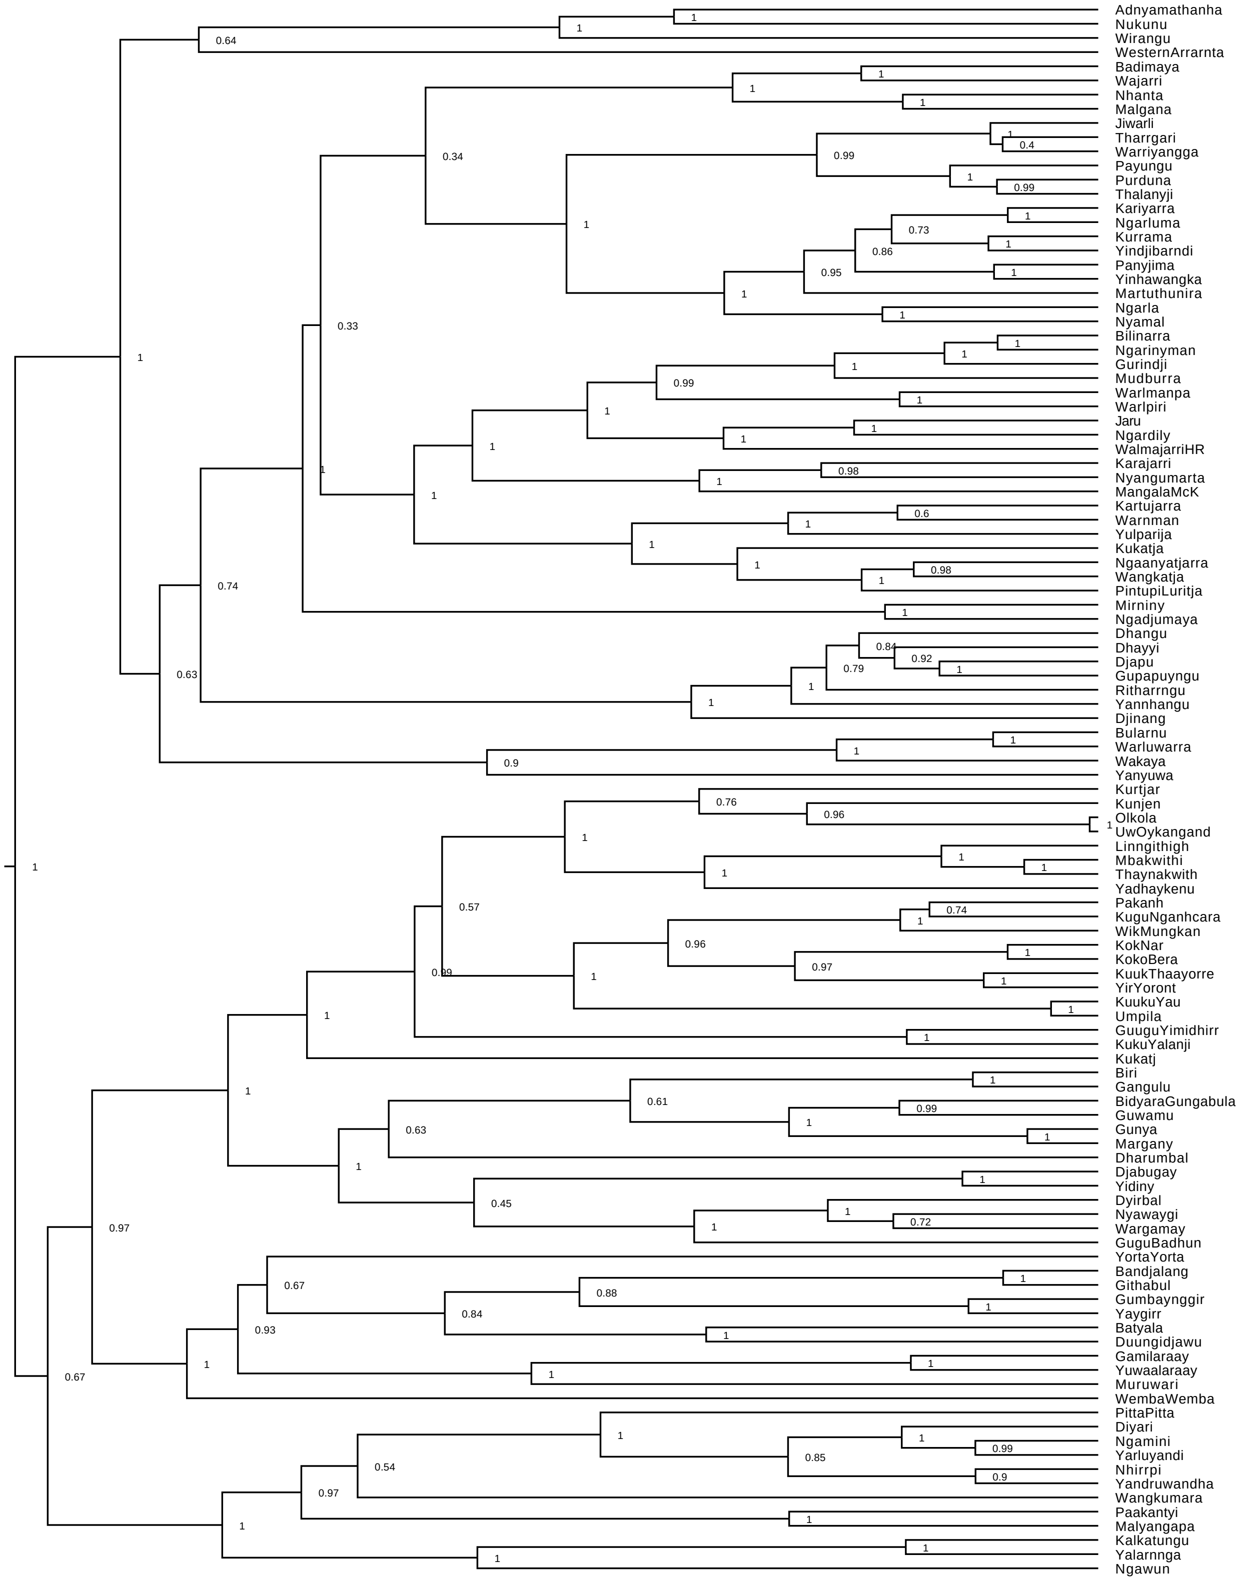


Figure S1. Pama-Nyungan reference phylogeny. Node labels are posterior probabilities, giving an indication of support for each node. Although there is no strict, conventional cut-off, clades with posterior values above 0.5 are considered supported and values above 0.8 are considered strongly supported (Bowern & Atkinson 2012, p.829).

## S2. Wordlist sources

The 111 wordlists used in this study are contained within the Ausphonlex database, under development by Round (2017). All underlying wordlist data is available, either publicly in the CHIRILA database (Bowern 2016) or elsewhere in published or archived form. A list of original sources for all wordlists is presented below.

**Adnyamathanha**

CHIRILA source: CHIRILA/v2/McEnteeMcKenzie

John McEntee & Pearl McKenzie. 1992. *Adna-mat-na English dictionary.* Adelaide: the authors. 125 pp.

Phonemic normalization: Coda tap normalized as vibrant. Otherwise, voiced stops, taps and fricatives normalized to lenis obstruents.

**Mbakwithi**

CHIRILA source: CHIRILA/v1/ASEDA0240

Terry Crowley. 1989. Mbakwithi vocabulary. Australian Institute of Aboriginal and Torres Strait Islander Studies, Australian Indigenous Languages Collection. ASEDA 0240. Canberra

**Badimaya**

Doug Marmion. 1995. Badimaya dictionary. Australian Institute of Aboriginal and Torres Strait Islander Studies, Australian Indigenous Languages Collection. ASEDA 0615. Canberra

Phonemic normalization: Double a normalized to long vowel.

**Pakanh**

Philip Hamilton. 1997a. *Pakanh Alphabetical Search Index.* Oykangand and Olkola Dictionary. http://www.oocities.org/athens/delphi/2970/pakalpha.htm

**BidyaraGungabula**

Gavan Breen. 1973. *Bidyara and Gungabula grammar and vocabulary.* Vol. 8 (Linguistic Communications). Melbourne: Monash University. 227 pp.

**Bilinarra**

Felicity Meakins, Lauren Campbell, et al. 2013. *Bilinarra to English dictionary.* Batchelor, NT, Australia: Batchelor Press. 264 pp.

**Biri**

CHIRILA source: CHIRILA/v1/Terrell

Angela Terrill. 1999. Biri lexicons. Australian Institute of Aboriginal and Torres Strait Islander Studies, Australian Indigenous Languages Collection. ASEDA 0700. Canberra. http://aiatsis.gov.au/sites/default/files/catalogue_resources/0700_access.zip

**Bularnu**

Gavan Breen. 1988. Bularnu grammar and vocabulary machine-readable files. Australian Institute of Aboriginal and Torres Strait Islander Studies, Australian Indigenous Languages Collection. ASEDA 0007. Canberra. http://aiatsis.gov.au/sites/default/files/catalogue_resources/0007_access.zip

**Batyala**

Jeanie Bell. 2003. *A sketch grammar of the Badjala language of Gari (Fraser Island).* Melbourne: University of Melbourne M.A. Thesis

**Dhangu**

R. David Zorc. 2004. Yolngu Matha dictionary. Australian Institute of Aboriginal and Torres Strait Islander Studies, Australian Indigenous Languages Collection. ASEDA 0778. Canberra. http://aiatsis.gov.au/sites/default/files/catalogue_resources/0778_Access.zip

Phonemic normalization: Lenis retroflex stop normalized to retroflex flap.

**Dharumbal**

CHIRILA source: CHIRILA/v2/ter02

Angela Terrill. 2002. *Dharumbal: the language of Rockhampton, Australia* (Pacific Linguistics 525). Canberra: Pacific Linguistics. 108 pp. https://doi.org/10.15144/PL-525

**Dhayyi**

Djarrayang Wunungmurra. 1993. Dhalwangu dictionary. Australian Institute of Aboriginal and Torres Strait Islander Studies, Australian Indigenous Languages Collection. ASEDA 0502. Canberra

Phonemic normalization: Lenis retroflex stop normalized to retroflex flap; all other voicing is allophonic.

**Diyari**

Peter K. Austin. 1981. *A grammar of Diyari, South Australia* (Cambridge Studies in Linguistics 32). Cambridge; New York: Cambridge University Press. 269 pp.

Phonemic normalization: Phonetic trill-released stop normalized as stop + trill. Otherwise, voiced stops normalized as taps.

**Djabugay**

Sue Robertson & Bruce A. Sommer. 1997. Jaabugay dictionary. Australian Institute of Aboriginal and Torres Strait Islander Studies, Australian Indigenous Languages Collection. ASEDA 0013. Canberra

**Djapu**

CHIRILA source: CHIRILA/v1/mor83

Frances Morphy. 1983. Djapu, a Yolngu dialect. In R. M. W. Dixon & Barry Blake (eds.), *Handbook of Australian languages*, vol. 3, 5 vols., 1–188. Amsterdam: John Benjamins

Phonemic normalization: Lenis retroflex stop normalized to retroflex flap.

**Djinang**

CHIRILA source: CHIRILA/v1/ASEDA0009

Bruce E. Waters. 1988. Djinang dictionary. Australian Institute of Aboriginal and Torres Strait Islander Studies, Australian Indigenous Languages Collection. ASEDA 0009. Canberra

Phonemic normalization: Glottal closure normalized to a segment phoneme.

**Duungidjawu**

CHIRILA source: CHIRILA/v2/K&W 04

Suzanne Kite & Stephen A. Wurm. 2004. *The Duungidjawu language of southeast Queensland: grammar, texts and vocabulary* (Pacific Linguistics 553). Canberra: Pacific Linguistics. 298 pp. https://doi.org/10.15144/PL-553

**Dyirbal**

CHIRILA source: CHIRILA/v1/dix72

R. M. W. Dixon. 1972. *The Dyirbal language of North Queensland.* Cambridge: Cambridge University Press

**Gamilaraay**

CHIRILA source: CHIRILA/v1/ash03

Anna Ash, John Giacon & Amanda Lissarrague. 2003. *Gamilaraay, Yuwaalaraay & Yuwaalayaay dictionary.* Alice Springs, NT, Australia: IAD Press. 344 pp.

**Gangulu**

CHIRILA source: CHIRILA/v1/Terrell

Angela Terrill. 1999. Biri lexicons. Australian Institute of Aboriginal and Torres Strait Islander Studies, Australian Indigenous Languages Collection. ASEDA 0700. Canberra. http://aiatsis.gov.au/sites/default/files/catalogue_resources/0700_access.zip

**Githabul**

CHIRILA source: CHIRILA/v1/cro78

Terry Crowley. 1978. *The Middle Clarence dialects of Bandjalang.* Vol. 12 (Research and regional studies). Canberra: Australian Institute of Aboriginal Studies

**GuguBadhun**

CHIRILA source: CHIRILA/v1/sut73

Peter John Sutton. 1973. Gugu-Badhun and its neighbours. In *Gugu-Badhun and its neighbours: a linguistic salvage study*, 24–67. Sydney: Macquarie University

**Gumbaynggir**

Murrbay Aboriginal and Culture Cooperative. 2001. *A Gumbaynggir language dictionary = Gumbayngirr bijarr jandaygam.* Canberra: Aboriginal Studies Press. 160 pp.

**Gunya**

CHIRILA source: CHIRILA/v1/dixbla81

Gavan Breen. 1981a. Margany and Gunya. In R. M. W. Dixon & Barry Blake (eds.), *Handbook of Australian languages*, vol. 2, 275–394. Amsterdam: John Benjamins

**Gupapuyngu**

CHIRILA source: CHIRILA/v1/BL

Beulah Lowe & Beulah Lowe. 1976. Temporary Gupapuyngu dictionary. Milingimbi, NT, Australia

**Gurindji**

Felicity Meakins, Patrick McConvell, et al. 2013. *Gurindji to English dictionary.* Batchelor, NT, Australia: Batchelor Press. 596 pp.

**GuuguYimidhirr**

John B. Haviland. 1979. Guugu Yimidhirr. In R. M. W. Dixon & Barry Blake (eds.), *Handbook of Australian languages*, vol. 1, 5 vols., 26–180. Amsterdam: John Benjamins

**Guwamu**

CHIRILA source: CHIRILA/v1/Austin 1980

Peter K. Austin. 1980. Guwamu vocabulary and English-Guwamu finder list. Cambridge, MA

**Jaru**

Tasaku Tsunoda. 1981. Jaru wordlist. In David Nash (ed.). In collab. with Kathleen Menning, Joyce Hudson & G Cooling, *Sourcebook for Central Australian languages.* ASEDA 0119. Alice Springs, NT, Australia: Institute for Aboriginal Development

Phonemic normalization: iji and uwu normalized as long high vowels.

**Jiwarli**

CHIRILA source: CHIRILA/v2/ASEDA0435

Peter K. Austin. N.d.(a). A dictionary of Jiwarli. Australian Institute of Aboriginal and Torres Strait Islander Studies, Australian Indigenous Languages Collection. ASEDA 0435. Canberra

**Kalkatungu**

CHIRILA source: CHIRILA/v2/ASEDA0205

Barry J. Blake. 1990a. Kalkatungu vocabulary. Australian Institute of Aboriginal and Torres Strait Islander Studies, Australian Indigenous Languages Collection. ASEDA 0205. Canberra

Phonemic normalization: Double short vowels normalized as long.

**Karajarri**

Kevin R. McKelson. 1989. Studies in Karajarri. grammatical sketch and dictionary

**Kariyarra**

Sue Smythe & Manny Lockyer. N.d. Kariyarra wordlist. Australian Institute of Aboriginal and Torres Strait Islander Studies, Australian Indigenous Languages Collection. ASEDA 0582. Canberra. http://aiatsis.gov.au/sites/default/files/catalogue_resources/0582_access.zip

**Kartujarra**

Geoffrey N. O'Grady. 1988a. Gardudjarra wordlist. Australian Institute of Aboriginal and Torres Strait Islander Studies, Australian Indigenous Languages Collection. ASEDA 0067. Canberra. http://aiatsis.gov.au/sites/default/files/catalogue_resources/0067_access.zip

**KokNar**

Bruce A. Sommer. N.d.(a). Koko Narr. Fryer Library Bruce Sommer Collection. UQFL476_b10f03_64, UQFL476_b10f03_65. Brisbane

**KokoBera**

Paul D. Black & Kokoberrin Tribal Aboriginal Corporation. 2007. The Kokoberrin and their languages. Australian Institute of Aboriginal and Torres Strait Islander Studies, Australian Indigenous Languages Collection

**KuguNganhcara**

CHIRILA source: CHIRILA/v1/ASEDA0021

Ian Smith & Steve Johnson. 1989. Kugu Nganchara. Australian Institute of Aboriginal and Torres Strait Islander Studies, Australian Indigenous Languages Collection. ASEDA 0021. Canberra

**Kukatj**

Gavan Breen. 1991. Kukatj grammar machine-readable files. Australian Institute of Aboriginal and Torres Strait Islander Studies, Australian Indigenous Languages Collection. ASEDA 0022. Canberra. http://aiatsis.gov.au/sites/default/files/catalogue_resources/0022_access.zip

Phonemic normalization: Featureless vowel normalized as schwa.

**Kukatja**

CHIRILA source: CHIRILA/v1/ASEDA0504

Anthony Rex Peile & Hilaire Valiquette. N.d. A basic Kukatja to English dictionary. Australian Institute of Aboriginal and Torres Strait Islander Studies, Australian Indigenous Languages Collection. ASEDA 0504. Canberra

**KukuYalanji**

Henry D. Hershberger & Ruth Hershberger. 1986. *Kuku-Yalanji dictionary.* In collab. with Australian Aborigines Branch Summer Institute of Linguistics. Vol. 7 (Work Papers of SIL - AAIB. Series B). Darwin: Summer Institute of Linguistics, Australian Aborigines Branch. 294 pp.

**Kurrama**

Alan C. Dench. N.d. Kurrama. Australian Institute of Aboriginal and Torres Strait Islander Studies, Australian Indigenous Languages Collection. ASEDA 0481. Canberra. http://aiatsis.gov.au/sites/default/files/catalogue_resources/0481_access.zip

**Kurtjar**

CHIRILA source: CHIRILA/v1/ASEDA0026

Paul D. Black & Rolly Gilbert. 1988. Kurtjar dictionary. Australian Institute of Aboriginal and Torres Strait Islander Studies, Australian Indigenous Languages Collection. ASEDA 0026. Canberra

Phonemic normalization: Retroflex glide~tap normalized as glide.

**KuukuYau**

David A. Thompson. 1988. "sand beach" language: an outline of Kuuku Ya'u and Umpila. Australian Institute of Aboriginal and Torres Strait Islander Studies, Australian Indigenous Languages Collection. ASEDA 0027. Canberra

**Linngithigh**

Kenneth Hale. 1999. A Linngithigh vocabulary. Australian Institute of Aboriginal and Torres Strait Islander Studies, Australian Indigenous Languages Collection. ASEDA 0687. Canberra

Phonemic normalization: Trill-released stop normalized as stop + trill. Prenasalized stops normalized to nasal + lenis stop.

**Malgana**

Andrew Gargett. 2011. *A salvage grammar of Malgana, the language of Shark Bay, Western Australia* (Pacific Linguistics 624). Canberra: Pacific Linguistics. 102 pp. https://doi.org/10.15144/PL-624

**Malyangapa**

Luise A. Hercus. 1989. Maljangapa-Wadigali vocabulary. Australian Institute of Aboriginal and Torres Strait Islander Studies, Australian Indigenous Languages Collection. ASEDA 0246. Canberra. http://aiatsis.gov.au/sites/default/files/catalogue_resources/0246_access.zip

**MangalaMcK**

Kevin McKelson. 1989a. Mangala wordlist. Australian Institute of Aboriginal and Torres Strait Islander Studies, Australian Indigenous Languages Collection. ASEDA 0220. Canberra. http://aiatsis.gov.au/sites/default/files/catalogue_resources/0220_access.zip

**Margany**

CHIRILA source: CHIRILA/v1/bre81

Gavan Breen. 1981a. Margany and Gunya. In R. M. W. Dixon & Barry Blake (eds.), *Handbook of Australian languages*, vol. 2, 275–394. Amsterdam: John Benjamins

**Martuthunira**

Alan C. Dench. 1995. *Martuthunira, a language of the Pilbara region of Western Australia* (Pacific Linguistics Series C 125). Canberra: Pacific Linguistics. 406 pp. https://doi.org/10.15144/PL-C125

**Mirniny**

Geoffrey N. O'Grady & Edward M. Curr. 1988. Mirniny wordlist. Australian Institute of Aboriginal and Torres Strait Islander Studies, Australian Indigenous Languages Collection. ASEDA 0070. Canberra. http://aiatsis.gov.au/sites/default/files/catalogue_resources/0070_access.zip

**Mudburra**

David Nash et al. 1988. Mudburra wordlist. Australian Institute of Aboriginal and Torres Strait Islander Studies, Australian Indigenous Languages Collection. ASEDA 0031. Canberra. http://aiatsis.gov.au/sites/default/files/catalogue_resources/0031_access.zip

**Muruwari**

CHIRILA source: CHIRILA/v1/ASEDA0252

Lynette Frances Oates. 1992. *Muruwari (Moo-roo-warri) dictionary: words of an Aboriginal language of north-western New South Wales.* Albury, NSW, Australia: Graeme van Brummelen, produced with the assistance of the Australian Institute of Aboriginal & Torres Strait Islander Studies. 97 pp.

**Ngaanyatjarra**

Amee Glass. 1988. Ngaanyatjarra wordlist. Australian Institute of Aboriginal and Torres Strait Islander Studies, Australian Indigenous Languages Collection. ASEDA 0033. Canberra. http://aiatsis.gov.au/sites/default/files/catalogue_resources/0033_access.zip

**Ngadjumaya**

Wangka Maya Pilbara Aboriginal Language Centre. 2008. *Ngajumaya dictionary.* South Hedland, WA, Australia: Wangka Maya Pilbara Aboriginal Language Centre. 16 pp.

**Ngamini**

CHIRILA source: CHIRILA/v1/brendn

Gavan Breen. 1967. Ngamini material. Australian Institute of Aboriginal and Torres Strait Islander Studies, Australian Indigenous Languages Collection. MS 117. Canberra

Phonemic normalization: Phonetic trill-released stop normalized as stop + trill. Otherwise, voiced stops normalized as taps.

**Ngardily**

Thomas M. Green. 1988. Ngardily wordlist. Australian Institute of Aboriginal and Torres Strait Islander Studies, Australian Indigenous Languages Collection. ASEDA 0034. Canberra. http://aiatsis.gov.au/sites/default/files/catalogue_resources/0034_access.zip

**Ngarinyman**

Caroline Jones. 2005. Ngarinman vocabulary. Australian Institute of Aboriginal and Torres Strait Islander Studies, Australian Indigenous Languages Collection. ASEDA 0796. Canberra

**Ngarla**

Alexander Brown & Brian Geytenbeek. N.d. Ngarla-English dictionary (interim), English-Ngarla wordlist. Australian Institute of Aboriginal and Torres Strait Islander Studies, Australian Indigenous Languages Collection. ASEDA 0060. Canberra

**Ngarluma**

Kenneth Hale. 1989. Ngarluma wordlist. Australian Institute of Aboriginal and Torres Strait Islander Studies, Australian Indigenous Languages Collection. ASEDA 0037. Canberra. http://aiatsis.gov.au/sites/default/files/catalogue_resources/0037_access.zip

**Ngawun**

CHIRILA source: CHIRILA/v2/BreenMayi

Gavan Breen. 1981b. *The Mayi languages of the Queensland Gulf Country* (A.I.A.S. New Series 29). Canberra: Australian Institute of Aboriginal Studies. 238 pp.

**Nhanta**

CHIRILA source: CHIRILA/v1/ble01

Juliette Blevins. 2001. *Nhanda: an Aboriginal language of Western Australia* (Oceanic linguistics special publication 30). Honolulu: University of Hawai'i Press. 170 pp.

**Yannhangu**

CHIRILA source: CHIRILA/v1/CB-fieldnotes

Bentley James. 2003. *Yan-nhangu dictionary.* In collab. with Laurie Baymarrwanga et al. Milingimbi, NT, Australia: B. James. 34 pp.

**Nhirrpi**

CHIRILA source: CHIRILA/v1/bow-nhi

Claire Bowern. 1999. Nhirrpi vocabulary, based on fieldnotes of S. A. Wurm

**Nukunu**

CHIRILA source: CHIRILA/v2/her92

Luise A. Hercus. 1992a. *A Nukunu dictionary.* Canberra: Department of Linguistics, Australian National University. 51 pp.

Phonemic normalization: Voiced retroflex stop normalized to retroflex tap.

**Nyamal**

Albert Burgman. 2007b. *Nyamal dictionary: English-Nyamal finderlist and topical wordlist.* In collab. with Wangka Maya Pilbara Aboriginal Language Centre. South Hedland, WA, Australia: Wangka Maya Pilbara Aboriginal Language Centre. 59 pp.

**Nyangumarta**

Brian Geytenbeek, Helen Geytenbeek & Wangka Maya Pilbara Aboriginal Language Centre. 1991. *Nyangumarta-English dictionary (interim), with an English-Nyangumarta finder list.* Port Hedland, WA, Australia: Wangka Maya Pilbara Aboriginal Language Centre. 119 pp.

**Nyawaygi**

R. M. W. Dixon. 1983. Nyawaygi. In R. M. W. Dixon & Barry J. Blake (eds.), *Handbook of Australian languages*, vol. 3, 5 vols., 431–531. Amsterdam: John Benjamins

**Kunjen**

Bruce A. Sommer. N.d.(b). Ogh Unydjan. Fryer Library Bruce Sommer Collection. UQFL476_b09f03_s05. Brisbane

**Olkola**

Philip Hamilton. 1997b. *Uw Olkola and Uw Oykangand Alphabetical Search Index.* Oykangand and Olkola Multimedia Dictionary. http://www.oocities.org/athens/delphi/2970/olkola.htm

**UwOykangand**

Philip Hamilton. 1997b. *Uw Olkola and Uw Oykangand Alphabetical Search Index.* Oykangand and Olkola Multimedia Dictionary. http://www.oocities.org/athens/delphi/2970/olkola.htm

**Panyjima**

Alan C. Dench. 1991. Panyjima. Australian Institute of Aboriginal and Torres Strait Islander Studies, Australian Indigenous Languages Collection. ASEDA 0375. Canberra. http://aiatsis.gov.au/sites/default/files/catalogue_resources/0375_access.zip

**Payungu**

CHIRILA source: CHIRILA/v1/ASEDA0394

Peter K. Austin. N.d.(d). Payungu - English dictionary. Australian Institute of Aboriginal and Torres Strait Islander Studies, Australian Indigenous Languages Collection. ASEDA 0394. Canberra

**PintupiLuritja**

Kenneth Hansen & Lesley Hansen. 1992. *Pintupi/Luritja dictionary.* 3rd edn. Alice Springs, NT, Australia: Institute for Aboriginal Development. 267 pp.

**PittaPitta**

CHIRILA source: CHIRILA/v1/bla0275

Barry J. Blake. 1990b. Pitta Pitta wordlist. Australian Institute of Aboriginal and Torres Strait Islander Studies, Australian Indigenous Languages Collection. ASEDA 0275. Canberra

**Purduna**

Albert Burgman. 2007a. *Burduna dictionary: English-Burduna wordlist and thematic wordlist.* In collab. with Wangka Maya Pilbara Aboriginal Language Centre. South Hedland, WA, Australia: Wangka Maya Pilbara Aboriginal Language Centre. 86 pp.

**Ritharrngu**

CHIRILA source: CHIRILA/v1/Heath

Jeffrey Heath. 1976. Ritharngu. In R. M. W. Dixon (ed.), *Grammatical categories in australian languages* (Linguistic series 22), 285–287. Canberra: Australian Institute of Aboriginal Studies

**Paakantyi**

Luise A. Hercus. N.d.(a). Paakantyi dictionary. Australian Institute of Aboriginal and Torres Strait Islander Studies, Australian Indigenous Languages Collection. ASEDA 0525. Canberra. http://aiatsis.gov.au/sites/default/files/catalogue_resources/0525_access.zip

**KuukThaayorre**

Tom Foote & Allen Hall. 1993. *Kuuk Thaayorre dictionary: Thaayorre/English ; september, 1966-92.* Brisbane: Jolien Press. 239 pp.

**Thalanyji**

CHIRILA source: CHIRILA/v2/ASEDA0437

Peter K. Austin. N.d.(b). A dictionary of Thalanyji. Australian Institute of Aboriginal and Torres Strait Islander Studies, Australian Indigenous Languages Collection. ASEDA 0437. Canberra

**Tharrgari**

Peter K. Austin. 1992. *A dictionary of Tharrgari, Western Australia.* Bundoora, Victoria, Australia: La Trobe University. 60 pp.

**Thaynakwith**

Gloria Thancoupie Fletcher. 2007. *Thanakupi's guide to language and culture: a Thaynakwith dictionary.* North Sydney, NSW, Australia: Jennifer Isaacs Arts & Publishing. 144 pp.

**Umpila**

Geoffrey N. O'Grady. 1988b. Umpila wordlist. Australian Institute of Aboriginal and Torres Strait Islander Studies, Australian Indigenous Languages Collection. ASEDA 0094. Canberra. http://aiatsis.gov.au/sites/default/files/catalogue_resources/0094_access.zip

**Bandjalang**

CHIRILA source: CHIRILA/v1/cro78

Terry Crowley. 1978. *The Middle Clarence dialects of Bandjalang.* Vol. 12 (Research and regional studies). Canberra: Australian Institute of Aboriginal Studies

**WalmajarriHR**

Joyce Hudson & Eirlys Richards. 1993. Walmajarri dictionary. Australian Institute of Aboriginal and Torres Strait Islander Studies, Australian Indigenous Languages Collection. ASEDA 0167. Canberra

**Wangkatja**

Noel Blyth. 2001. Wangka dictionary and grammar. Australian Institute of Aboriginal and Torres Strait Islander Studies, Australian Indigenous Languages Collection. ASEDA 0709. Canberra. http://aiatsis.gov.au/sites/default/files/catalogue_resources/0709_access.zip

**Wangkumara**

CHIRILA source: CHIRILA/v1/robnd

Carol Robertson. 1985. *Wangkumara grammar and dictionary.* Sydney: Department of Technical & Further Education, Aboriginal Education Unit. 90 pp.

Phonemic normalization: Double a normalized to long vowel.

**Warlmanpa**

David Nash, Kenneth Hale & Gavan Breen. 1984. Preliminary vocabulary of Warlmanpa. Australian Institute of Aboriginal and Torres Strait Islander Studies, Australian Indigenous Languages Collection. ASEDA 0049. Canberra

**Warlpiri**

CHIRILA source: CHIRILA/v2/WarlpiriDict

Steve Schwartz. 1996. Warlpiri draft dictionary

**Warluwarra**

Gavan Breen. 1990. Warluwara grammar and wordlist. Australian Institute of Aboriginal and Torres Strait Islander Studies, Australian Indigenous Languages Collection. ASEDA 0253. Canberra

Phonemic normalization: Prenasalized stops normalized to nasal + lenis stop. Tense glides normalized to fricatives. Tense lateral normalized to double lateral.

**Warnman**

CHIRILA source: CHIRILA/v2/ASEDA0334

Wangka Maya Pilbara Aboriginal Language Centre. N.d. Warnman wordlist. Australian Institute of Aboriginal and Torres Strait Islander Studies, Australian Indigenous Languages Collection. ASEDA 0334. Canberra. http://aiatsis.gov.au/sites/default/files/catalogue_resources/0334_Access.zip

**Wargamay**

CHIRILA source: CHIRILA/v1/dixbla81

R. M. W. Dixon. 1981. Wargamay. In R. M. W. Dixon & Barry Blake (eds.), *Handbook of Australian languages*, vol. 2, 5 vols., 1–145. Amsterdam: John Benjamins

**Warriyangga**

Peter K. Austin. N.d.(c). A dictionary of Warriyangka. Australian Institute of Aboriginal and Torres Strait Islander Studies, Australian Indigenous Languages Collection. ASEDA 0439. Canberra

**Wajarri**

Doreen Mackman (ed.). 2012. *Wajarri dictionary: the language of the Murchison Region of Western Australia.* In collab. with Irra Wangga Language Centre & Yamaji Language Aboriginal Corporation. Geraldton, WA, Australia: Irra Wangga Language Centre. 249 pp. http://www.bundiyarra.com.au/wajarriApp/ (23 July, 2018)

**WembaWemba**

Luise A. Hercus. 1992b. *Wembawemba dictionary.* Canberra: L.A. Hercus. 116 pp.

**WesternArrarnta**

Gavan Breen. 2000. *Introductory dictionary of Western Arrernte.* In collab. with John Pfitzner. Alice Springs, NT, Australia: IAD Press. 120 pp.

Phonemic normalization: Labialized consonants normalized to C + w. Prestopped nasals normalized to stop + nasal sequence. Prepalatalized consonants normalized to j + C.

**Wakaya**

Gavan Breen. 2006. Wakaya. Australian Institute of Aboriginal and Torres Strait Islander Studies, Australian Indigenous Languages Collection. ASEDA 0047. Canberra. http://aiatsis.gov.au/sites/default/files/catalogue_resources/0047_access.zip (30 July, 2018)

**WikMungkan**

Christine Kilham et al. 2011. *Wik Mungkan-English Interactive Dictionary.* AuSIL Interactive Dictionary Series A-6. In collab. with Charles E. Grimes & Maarten Lecompte. http://ausil.org/Dictionary/Wik-Mungkan/lexicon/mainintro.htm (26 July, 2018)

**Wirangu**

Luise A. Hercus. 1999. *A grammar of the Wirangu language from the West Coast of South Australia* (Pacific Linguistics Series C 150). Canberra: Pacific Linguistics. 239 pp. https://doi.org/10.15144/PL-C150

Phonemic normalization: Double a normalized to long vowel.

**Yadhaykenu**

Terry Crowley. 1983. Uradhi. In R. M. W. Dixon & Barry J. Blake (eds.), *Handbook of Australian languages*, vol. 3, 5 vols., 307–428. Amsterdam: John Benjamins

**Yalarnnga**

CHIRILA source: CHIRILA/v1/ASEDA0204

Gavan Breen & Barry J Blake. N.d. Yalarnnga vocab. Australian Institute of Aboriginal and Torres Strait Islander Studies, Australian Indigenous Languages Collection. ASEDA 0204. Canberra

**Yandruwandha**

CHIRILA source: CHIRILA/v1/breyandr

Gavan Breen. 2004. *Innamincka talk: a grammar of the Innamincka dialect of Yandruwandha with notes on other dialects* (Pacific Linguistics 558). Canberra: Pacific Linguistics. 245 pp. https://doi.org/10.15144/PL-558

Phonemic normalization: Trill-released stop normalized as stop + trill. Prestopped laterals normalized to stop + lateral sequence.

**Yanyuwa**

John Bradley. N.d. Yanyuwa dictionary. Australian Institute of Aboriginal and Torres Strait Islander Studies, Australian Indigenous Languages Collection. ASEDA 0382. Canberra

Phonemic normalization: Prenasalized stops normalized to nasal + stop sequence.

**Yarluyandi**

CHIRILA source: CHIRILA/v1/ASEDA0251

Luise A. Hercus. N.d.(b). Yarluyandi vocabulary. Australian Institute of Aboriginal and Torres Strait Islander Studies, Australian Indigenous Languages Collection. ASEDA 0251. Canberra. http://aiatsis.gov.au/sites/default/files/catalogue_resources/0251_access.zip

**Yaygirr**

CHIRILA source: CHIRILA/v1/morelli2011

Steve Morelli. 2012. *Yaygirr dictionary and grammar*. In collab. with Many Rivers Aboriginal Language Centre. Nambucca Heads, NSW, Australia: Muurrbay Aboriginal Language & Culture Co-operative. 254 pp.

**Yidiny**

CHIRILA source: CHIRILA/v2/dix91

R. M. W. Dixon. 1991. *Words of our country: stories, place names, and vocabulary in Yidiny, the Aboriginal language of the Cairns-Yarrabah region*. In collab. with Tony Irvine. St Lucia, Qld: University of Queensland Press. 312 pp.

**Yindjibarndi**

Bruce Anderson, E. Richards & Summer Institute of Linguistics. N.d. Yindjibarndi dictionary. Australian Institute of Aboriginal and Torres Strait Islander Studies, Australian Indigenous Languages Collection. ASEDA 0297. Canberra. http://aiatsis.gov.au/sites/default/files/catalogue_resources/0297_access.zip

**Yinhawangka**

Wangka Maya Pilbara Aboriginal Language Centre. 2008. *Yinhawangka dictionary: English-Yinhawangka wordlist and topical wordlists 2008: draft 1*. South Hedland, WA, Australia: Wangka Maya Pilbara Aboriginal Language Centre. 92 pp.

**YirYoront**

Barry Alpher. 1991. *Yir-Yoront lexicon: sketch and dictionary of an Australian language*. Vol. 6 (Trends in Linguistics: Documentation). Berlin, New York: Mouton de Gruyter

**YortaYorta**

CHIRILA source: CHIRILA/v1/bowmor99

Heather Bowe & Stephen Morey. 1999. *The Yorta Yorta (Bangerang) language of the Murray Goulburn including Yabula Yabula* (Pacific Linguistics Series C 154). Canberra: Pacific Linguistics. 286 pp.

**Yulparija**

Kevin McKelson. 1989b. Yulparija. Australian Institute of Aboriginal and Torres Strait Islander Studies, Australian Indigenous Languages Collection. ASEDA 0032. Canberra. http://aiatsis.gov.au/sites/default/files/catalogue_resources/0032_access.zip

**Yuwaalaraay**

CHIRILA source: CHIRILA/v1/ash03

Anna Ash, John Giacon & Amanda Lissarrague. 2003. *Gamilaraay, Yuwaalaraay & Yuwaalayaay dictionary*. Alice Springs, NT, Australia: IAD Press. 344 pp.

## S3. Guide to code and data

The code and data used in this study are publicly accessible on Zenodo at http://doi.org/10.5281/zenodo.3936353. Unzipping the file reveals a directory containing four subdirectories, `/trees`, `/data`, `/R`, and `/results`.

The `/trees` subdirectory contains two files: `PNY10_285.(time).sum.tree`, which is a Nexus format tree file for the Pama-Nyungan maximum clade credibility tree used as a reference tree throughout the study. `PNY10_285.trees` contains the full posterior sample of trees and was used to check the robustness of our results against phylogenetic uncertainty.

The `/data` subdirectory contains 9 comma-separated (csv) spreadsheets containing all the frequency data used in the study. In all cases, the first column lists language variety names and the first row lists characters (variables) for analysis. The `biphone_binary` spreadsheet contains binary permissibility data for the $D$ test for phylogenetic signal. A '1' value indicates that the biphone occurs at least once in that language variety's wordlist. A '0' indicates that the biphone never appears in the language variety's wordlist. A missing value (represented by 'NA') is entered where one or both of the phonological segments in the biphone is not part of the language variety's phonological inventory and therefore would be impossible to observe. The `biphone_fwd` and `biphone_bkwd` spreadsheets give the forward and backward transition probabilities for each language variety. Once again, missing values occur where the language lacks entirely one of the segments in a particular biphone. Otherwise, as discussed in the main paper body, the frequencies given are the frequencies of the sequency $xy$, relativised over all instances of $x$ (forward transition) or the frequencies of the sequency $xy$ relativised over all instances of $y$ (backward transition). The remaining spreadsheets give frequencies of transitions between natural sound classes. Natural classes are split into three categories, manner, place and major place. The format of the spreadsheet filenames is `{class type}_{transition direction}_{file creation date}.csv`. So, for example, the spreadsheet beginning with `place_fwd` gives the forward transition frequencies for transitions between places of articulation.

The `/R` subdirectory contains code used to perform the analysis for the study and create figures for the main text of the paper. The `analysis.R` script is written to run in *R* statistical software (R Core Team 2017). To run the analysis, the first step is to set the *R* working directory to the `/R` subdirectory. It is important to keep the file structure of the S2 directory intact, since the script requires access to the `data`, `trees` and `results` subdirectories. The first lines of the script load all its required packages. If any packages are missing from the machine, these will need to be installed. All packages used are standard packages available on the CRAN network (https://cran.r-project.org), and installation is straightforward using the `install.packages("package-name")` command in the R console. The script can be run from the R console using the command `source("analysis.R")`. It has been run succcessfully (approximately 45 minutes runtime) on a 2015 Macbook Pro with 8GB memory, with the following R session info:

```
R version 3.6.2 (2019-12-12)
Platform: x86_64-apple-darwin15.6.0 (64-bit)
Running under: macOS Catalina 10.15.4

Matrix products: default
BLAS:   /System/Library/Frameworks/Accelerate.framework/Versions/A/Frameworks/vecLib.framework/Versions/[illegible]
LAPACK: /Library/Frameworks/R.framework/Versions/3.6/Resources/lib/libRlapack.dylib

locale:
[1] en_AU.UTF-8/en_AU.UTF-8/en_AU.UTF-8/C/en_AU.UTF-8/en_AU.UTF-8

attached base packages:
[1] stats     graphics  grDevices utils     datasets  methods   base

other attached packages:
 [1] kSamples_1.2-9    SuppDists_1.1-9.5 phylosignal_1.3   phylobase_0.8.10
 [5] rcompanion_2.3.25 picante_1.8.1     nlme_3.1-145      vegan_2.5-6
```

```
 [9] lattice_0.20-40   permute_0.9-5     e1071_1.7-3       reshape2_1.4.3
[13] caper_1.0.1       mvtnorm_1.1-0     MASS_7.3-51.5     ape_5.3
[17] forcats_0.5.0     stringr_1.4.0     dplyr_0.8.4       purrr_0.3.3
[21] readr_1.3.1       tidyr_1.0.2       tibble_2.1.3      ggplot2_3.3.0
[25] tidyverse_1.3.0

loaded via a namespace (and not attached):
  [1] TH.data_1.0-10     colorspace_1.4-1   deldir_0.1-25      seqinr_3.6-1
  [5] class_7.3-15       modeltools_0.2-23  fs_1.3.2           rstudioapi_0.11
  [9] fansi_0.4.1        lubridate_1.7.4    coin_1.3-1         xml2_1.2.2
 [13] codetools_0.2-16   splines_3.6.2      libcoin_1.0-5      ade4_1.7-15
 [17] jsonlite_1.6.1     broom_0.5.5        cluster_2.1.0      dbplyr_1.4.2
 [21] shiny_1.4.0        compiler_3.6.2     httr_1.4.1         backports_1.1.5
 [25] assertthat_0.2.1   Matrix_1.2-18      fastmap_1.0.1      lazyeval_0.2.2
 [29] cli_2.0.2          later_1.0.0        htmltools_0.4.0    prettyunits_1.1.1
 [33] tools_3.6.2        igraph_1.2.4.2     coda_0.19-3        gtable_0.3.0
 [37] glue_1.3.1         gmodels_2.18.1     Rcpp_1.0.3         raster_3.0-12
 [41] cellranger_1.1.0   vctrs_0.2.3        spdep_1.1-3        gdata_2.18.0
 [45] lmtest_0.9-37      adephylo_1.1-11    rvest_0.3.5        mime_0.9
 [49] lifecycle_0.1.0    gtools_3.8.1       XML_3.99-0.3       LearnBayes_2.15.1
 [53] zoo_1.8-7          scales_1.1.0       hms_0.5.3          promises_1.1.0
 [57] parallel_3.6.2     sandwich_2.5-1     expm_0.999-4       EMT_1.1
 [61] stringi_1.4.6      nortest_1.0-4      boot_1.3-24        spData_0.3.3
 [65] rlang_0.4.5        pkgconfig_2.0.3    matrixStats_0.56.0 rncl_0.8.4
 [69] sf_0.8-1           tidyselect_1.0.0   plyr_1.8.6         magrittr_1.5
 [73] R6_2.4.1           DescTools_0.99.34  generics_0.0.2     multcompView_0.1-8
 [77] multcomp_1.4-12    DBI_1.1.0          pillar_1.4.3       haven_2.2.0
 [81] withr_2.1.2        mgcv_1.8-31        units_0.6-6        sp_1.4-1
 [85] survival_3.1-8     modelr_0.1.6       crayon_1.3.4       KernSmooth_2.23-16
 [89] uuid_0.1-4         progress_1.2.2     RNeXML_2.4.3       adegenet_2.1.2
 [93] grid_3.6.2         readxl_1.3.1       classInt_0.4-2     reprex_0.3.0
 [97] digest_0.6.25      xtable_1.8-4       httpuv_1.5.2       stats4_3.6.2
[101] munsell_0.5.0
```

Note that the `analysis.R` script contains the minimum script required to reproduce the analysis and output results files in the `/results` subdirectory. In addition, it contains a good deal of commented-out code that can be used for basic inspection of the results and production of summary statistics. This code can be uncommented or copied into the R console at user discretion. Runtime of the extra code is minimal, though it will produce a much more verbose output in R's console if run all at once.

The R script `modified_caper_funcs.R` contains some minimally-modified versions of functions in the `caper` package that are used in the $D$ test for phylogenetic signal in binary data. They have been tweaked to improve vectorisation of the original functions (in order to run the test over a large series of characters rather than a single character at a time). This script is read by the `analysis.R` script. Nothing needs to be done directly in the R console.

The script `tree_uncertainty.R` contains code for replicating part of the study (place and manner sound class characters) on a 100-tree subset of the posterior sample contained in `PN_SDollo.nex`. Its runtime is around 9.5 hours on the same machine described above. The script `wordlist_size_uncertainty.R` contains code for replicating the same part of the study on two subsets of languages: The middle 50% of wordlists when ranked by size and every 2nd wordlist when ranked by size. The runtime for this script is around 20 minutes. Note that due to random permutations in the methodology, exact replication is only possible if a random seed is set. To ensure the seed is set at the correct time, each script should be run in a clean R session. Alternatively, the analysis can be reproduced with new random numbers by changing or removing the `set.seed` command. Although we expect the overall results of the study to remain the same, there will

be slight differences in values that rely on stochastic processes for their calculation (for example, $p$ values that are calculated via bootstrapping).

Finally, the `create_figs.R` script contains code used to produce figures for the main text body. The script saves each figure as a PDF file in a `/fig` subdirectory (you will need to create this directory first, if it is not present already). Figures are produced with the `ggplot2` package, using the system of visualisation described by Wilkinson & Wills (2005).

The `/results` subdirectory contains original csv spreadsheets of results, generated as output from `analysis.R` and used in the study. Results from the $D$ test for phylogenetic signal in binary phonotactic data are contained in the spreadsheet `D_test_results_2020-06-06.csv`. The `biphone` column lists the biphone character tested. Note that the underscore in each biphone label is purely to aid readability and carries no linguistic meaning (it is not intended to look like the environment of a generative phonological rule). The `languages` column gives the number of languages with non-missing values for which phylogenetic signal was tested for that particular character. `count_0` and `count_1` columns give the number of observed 0 values and 1 values respectively. `D` gives the observed $D$ statistic for each character and the `pval_0` and `pval_1` columns give the uncorrected $p$ values for the two null hypotheses that $D = 0$ and $D = 1$ respectively. The columns `pval0_sig` and `pval1_sig` give text descriptions interpreting the significance of the $p$ values. If a $p$ value is small, the character will be either significantly more clumped or significantly more dispersed than the null hypothesis. Otherwise, the character will be consistent with the null hypothesis, either the phylogenetic null hypothesis ($D = 0$) or randomness null hypothesis ($D = 1$). Finally, the `result` column gives an overall interpretation of the result of the $D$ test and two accompanying $p$ values. There are six possible categories a character may fall into:

- (i) More clumped than the phylogenetic null hypothesis, listed as `more clumped`.
- (ii) consistent with the phylogenetic null hypothesis and more clumped than the random null hypothesis (i.e. there is significant phylogenetic signal), listed as `phylogenetic`.
- (iii) consistent with both null hypotheses, so a result cannot be determined either way, listed as `indeterminate (neither H0 rejected)`.
- (iv) inconsistent with both null hypotheses, and $0 < D < 1$, listed as `0 < D < 1 (both H0s rejected)`.
- (v) consistent with the randomness null hypothesis and more dispersed than the phylogenetic null hypothesis, listed as `random`.

The sixth possible category a character can fall into, which is written into the `analysis.R` script, is: more dispersed than the randomness null hypothesis, listed as `more dispersed`. However, in this study, we find no characters that fall into this category and thus it does not appear in the spreadsheet of results.

Results files for the $K$ tests are given in spreadsheets named according to the format `K_{character type}_{transition direction}_results_{date of analysis}_.csv`. There are four spreadsheets of results for biphone characters: Original forward and backward transition frequencies, and normalised forward and backward transition frequencies. For natural class-based characters, there are two spreadsheets corresponding to forward and backward transition frequencies for each of three class types: manner, place and major place.

The `\results` subdirectory also contains spreadsheets of results produced by `wordlist_size_uncertainty.R`. The results files obtained by taking every 2nd wordlist (when wordlists are ranked by size) are prefixed with `Every2nd`. The results files obtained by taking the middle 50% of wordlists are prefixed with `IQR` ('interquartile range'). The results of `tree_uncertainty.R` are saved as an `.Rdata` file which can be opened in R software. The file contains four list objects, each of length 100. The four lists contain results of $K$ tests applied to (i) forward transitions between manner classes, (ii) backward transitions between manner classes, (iii) forward transitions between place classes and (iv) backward transitions between place classes. Each of the 100 elements in each list corresponds to a tree in the Pama-Nyungan posterior tree sample. Each element contains a data frame giving the results of $K$ tests conducted on the applicable character set using a given tree in the posterior tree sample.

# References


Bouckaert, Remco R., Claire Bowern & Quentin D. Atkinson. 2018. The origin and expansion of Pama-Nyungan languages across Australia. *Nature Ecology & Evolution* 2(4). 741–749. https://doi.org/10.1038/s41559-018-0489-3.

Bouckaert, Remco R. et al. 2014. BEAST 2: a software platform for Bayesian evolutionary analysis. *PLoS Computational Biology* 10(4). e1003537. https://doi.org/10.1371/journal.pcbi.1003537.

Bowern, Claire. 2015. Pama-Nyungan phylogenetics and beyond [plenary address]. In *Lorentz center workshop on phylogenetic methods in linguistics*. Leiden University, Leiden, Netherlands. https://doi.org/10.5281/zenodo.3032846.

Bowern, Claire. 2016. Chirila: contemporary and historical resources for the indigenous languages of Australia. *Language Documentation and Conservation* 10. http://hdl.handle.net/10125/24685.

Bowern, Claire. 2018. *Pama-Nyungan cognate judgements: 285 languages*. 10.5281/zenodo.1318310.

Bowern, Claire & Quentin D. Atkinson. 2012. Computational phylogenetics and the internal structure of Pama-Nyungan. *Language* 88(4). 817–845. https://doi.org/10.1353/lan.2012.0081.

R Core Team. 2017. *R: a language and environment for statistical computing*. Vienna: R Foundation for Statistical Computing. https://www.R-project.org/.

Round, Erich R. 2017. The AusPhon-lexicon project: 2 million normalized segments across 300 Australian languages. In. Poznań, Poland.

Wilkinson, Leland & Graham Wills. 2005. *The grammar of graphics* (Statistics and Computing). New York: Springer.
