# Supplementary material for: Phylogenetic signal in phonotactics
Source: arXiv:2002.00527 source file (2020-07-14)
Supplement: Supplementary file 2 [file supplementary.tex]

\documentclass[]{article}
\pdfoutput=1
\usepackage{pdfpages}

\begin{document}
\includepdf[pages=1-last]{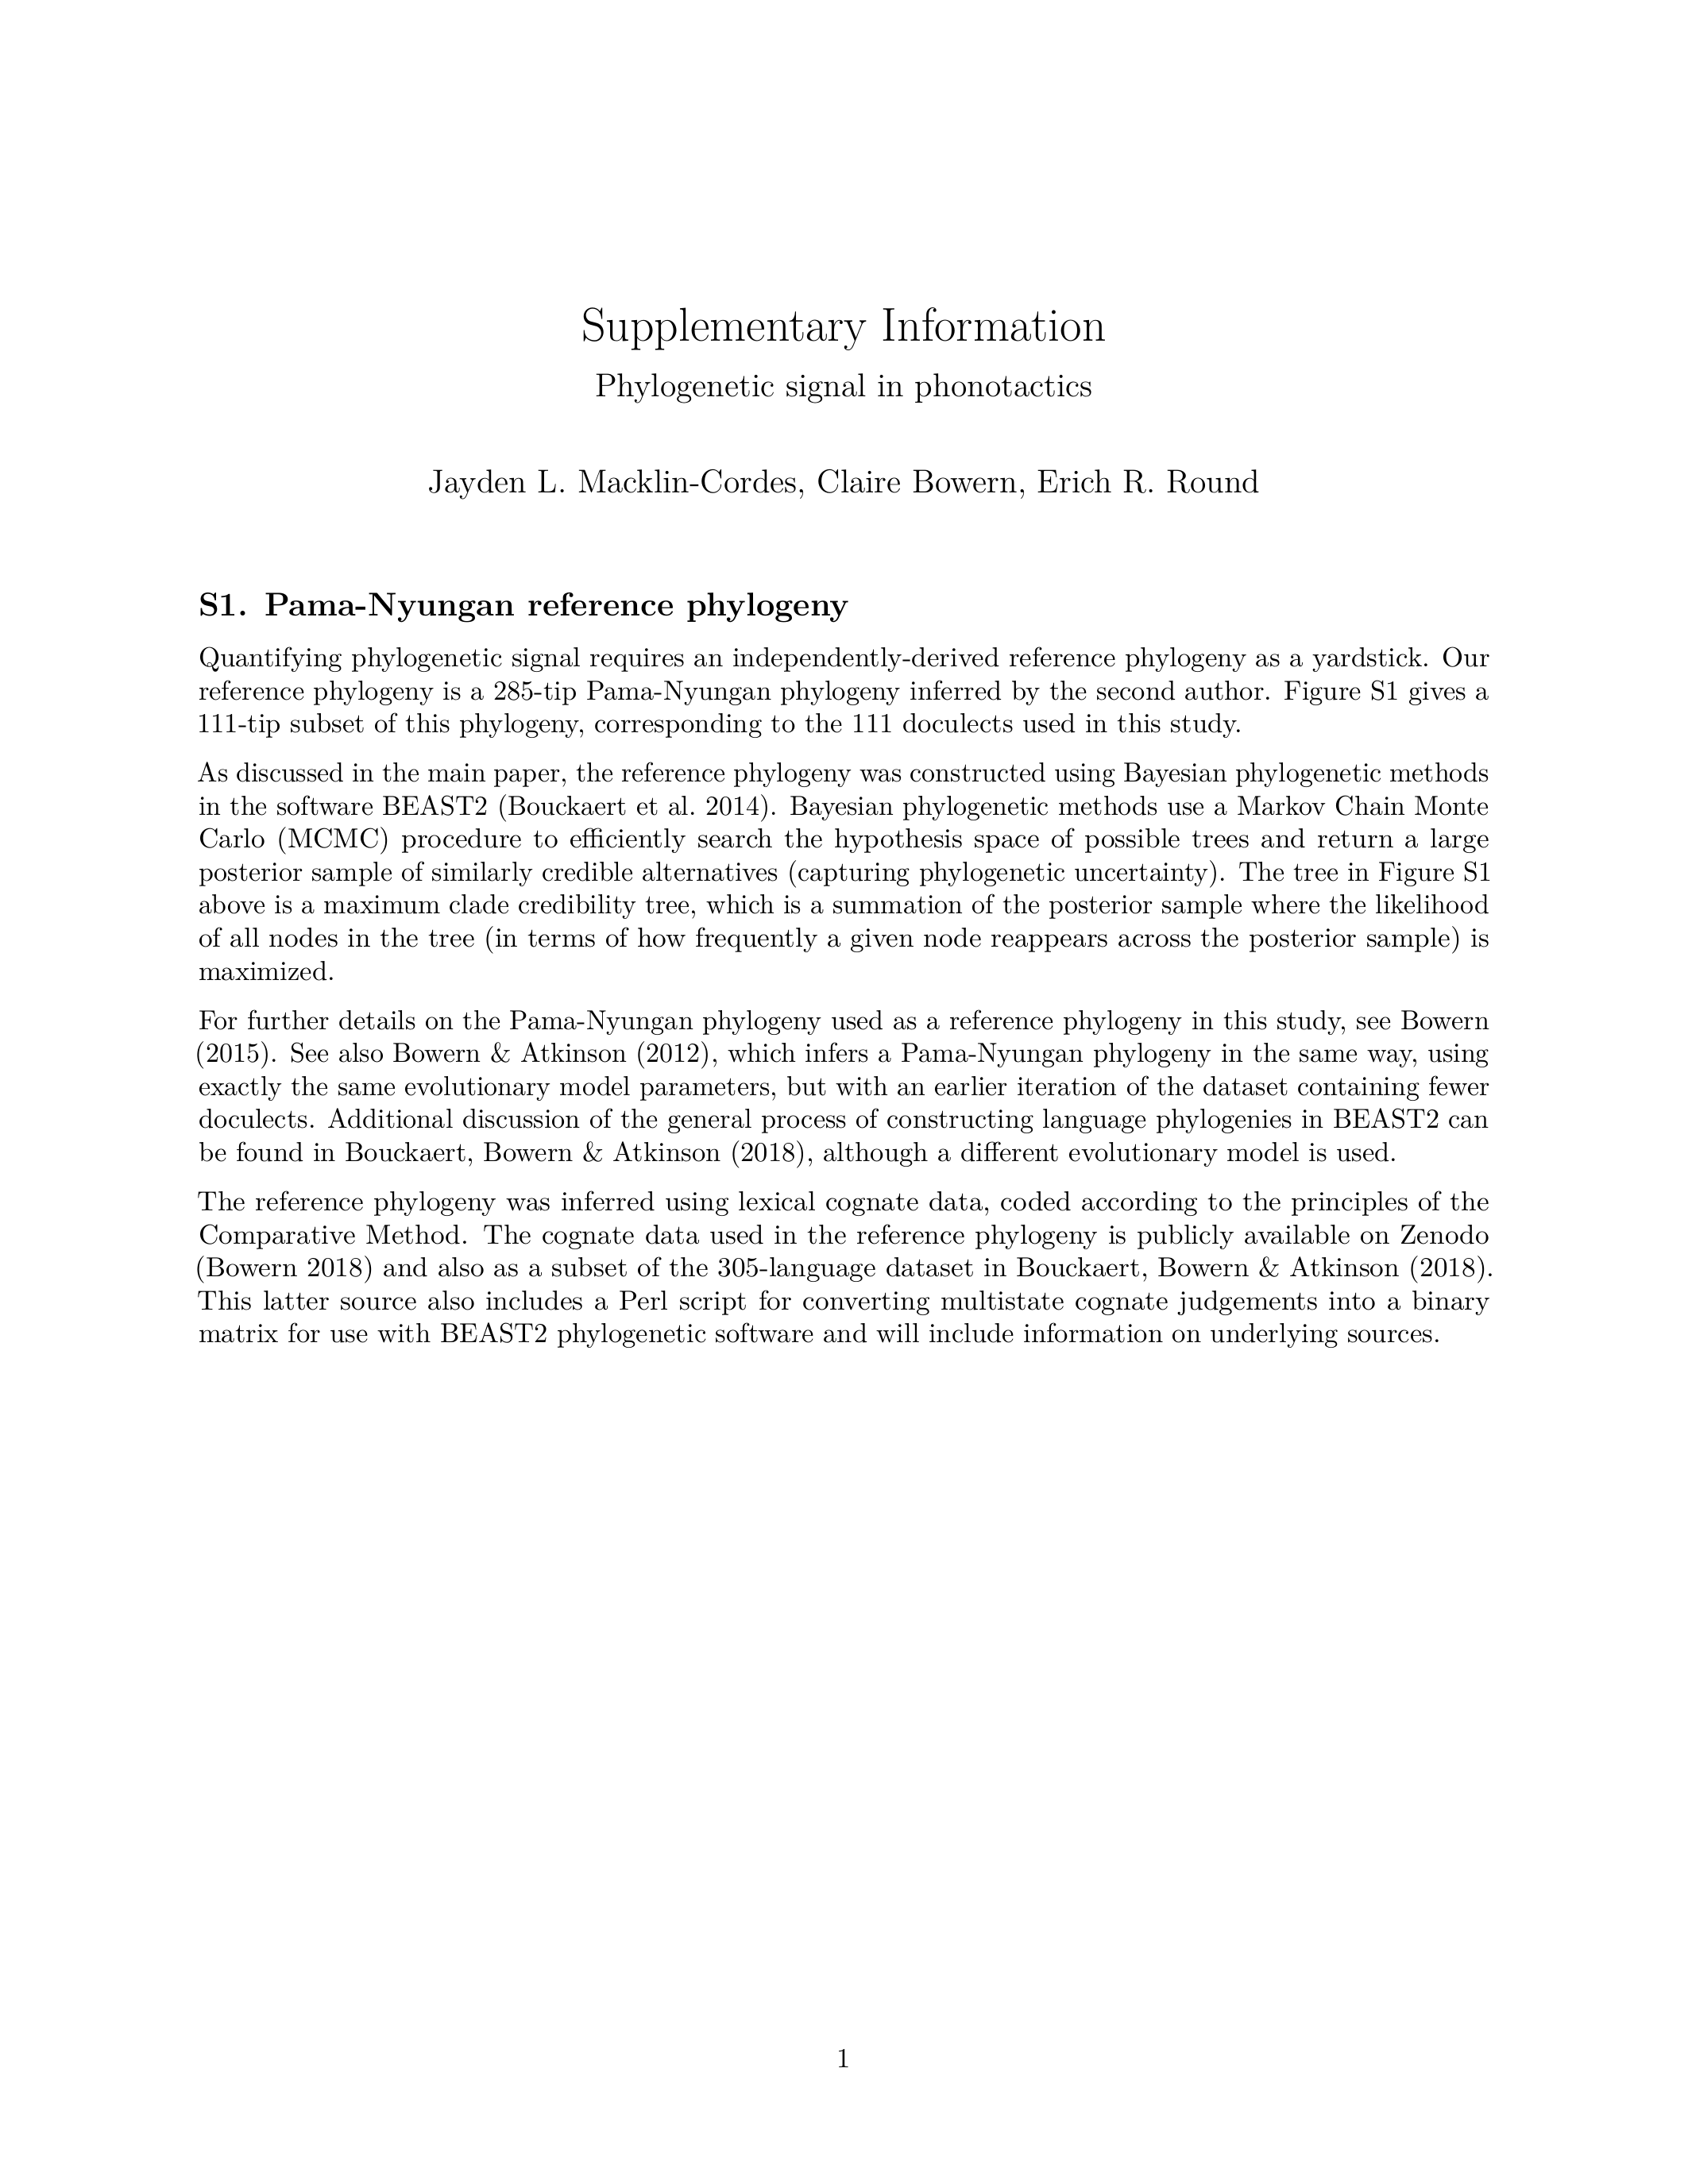}
\end{document}
